# Supplementary material for: DN-Splatter: Depth and Normal Priors for Gaussian Splatting and Meshing
Source: arXiv:2403.17822 source file (2024-11-07)
Supplement: Supplementary file 2 [file ab_normals.tex]

\begin{minipage}{1\linewidth}
  \centering
  \resizebox{\textwidth}{!}{%
        \begin{tabular}{cccccc}
          \hline
          Method & Acc $\downarrow$ & Comp $\downarrow$ & C-L1 $\downarrow$ & NC $\uparrow$ & F-score $\uparrow$ \\
          \hline
          Baseline (w/o $\mathcal{L}_{\hat{N}}$) & 0.87 & 3.33 & 2.10 & 91.54 & 92.52 \\
          Depth Gradient $\mathcal{L}_{\hat{N}}$ & 0.82 & 3.29 & 2.06 & 92.50 & 92.82 \\
          Monocular $\mathcal{L}_{\hat{N}}$  & \textbf{0.83} & \textbf{3.11} & \textbf{1.97} & \textbf{93.09} & \textbf{93.29} \\
          Monocular $\mathcal{L}_{\hat{N}} + \mathcal{L}_{\hat{N}_{smooth}}$ (Ours) & 0.86 & 3.12 & 1.99 & 92.92 & \textbf{93.29} \\ \hline
        \end{tabular}%
        }
        \label{tab:normal mesh metrics}
        \caption{Comparison of normal supervision on mesh quality.}
    \end{minipage}%
    
    \vspace{0em}
    \begin{minipage}{1\linewidth}
    \centering
    \label{tab:ablation-normal-loss}
    \resizebox{\textwidth}{!}{%
      \begin{tabular}{ccccc}
        \hline  & MAE (Rad) $\downarrow$ & MAE ($^{\circ}$) $\downarrow$ &  RMSE $\downarrow$ & Mean $\downarrow$ \\ 
        \hline
        Baseline (w/o $\mathcal{L}_{\hat{N}}$) & 0.509 & 29.17 & 0.342 & 0.249 \\
        Depth Gradient $\mathcal{L}_{\hat{N}}$ w/o $\mathcal{L}_{depth}$ & 0.383 & 21.95 & 0.282 & 0.189 \\
        Depth Gradient $\mathcal{L}_{\hat{N}}$ w/ $\mathcal{L}_{depth}$ & 0.239 & 13.74 & 0.203 & 0.118 \\
        Monocular $\mathcal{L}_{\hat{N}}$ &  0.103 & 5.89 & 0.099 & 0.046 \\
        Monocular $\mathcal{L}_{\hat{N}} + \mathcal{L}_{\hat{N}_{smooth}}$ (Ours) & \textbf{0.088} & \textbf{5.06} & \textbf{0.085} & \textbf{0.039} \\ \hline
      \end{tabular}
      }
      \caption{Comparison of normal supervision on rendered normals.}
    \end{minipage}
